# Supplementary material for: Learning SO(3)-Invariant Semantic Correspondence via Local Shape Transform
Source: arXiv:2404.11156 source file (2024-04-20)
Supplement: Supplementary file 1 [file supp_acceptance.tex]

\begin{figure}[h]
    \begin{center}
        \includegraphics[width=\linewidth]{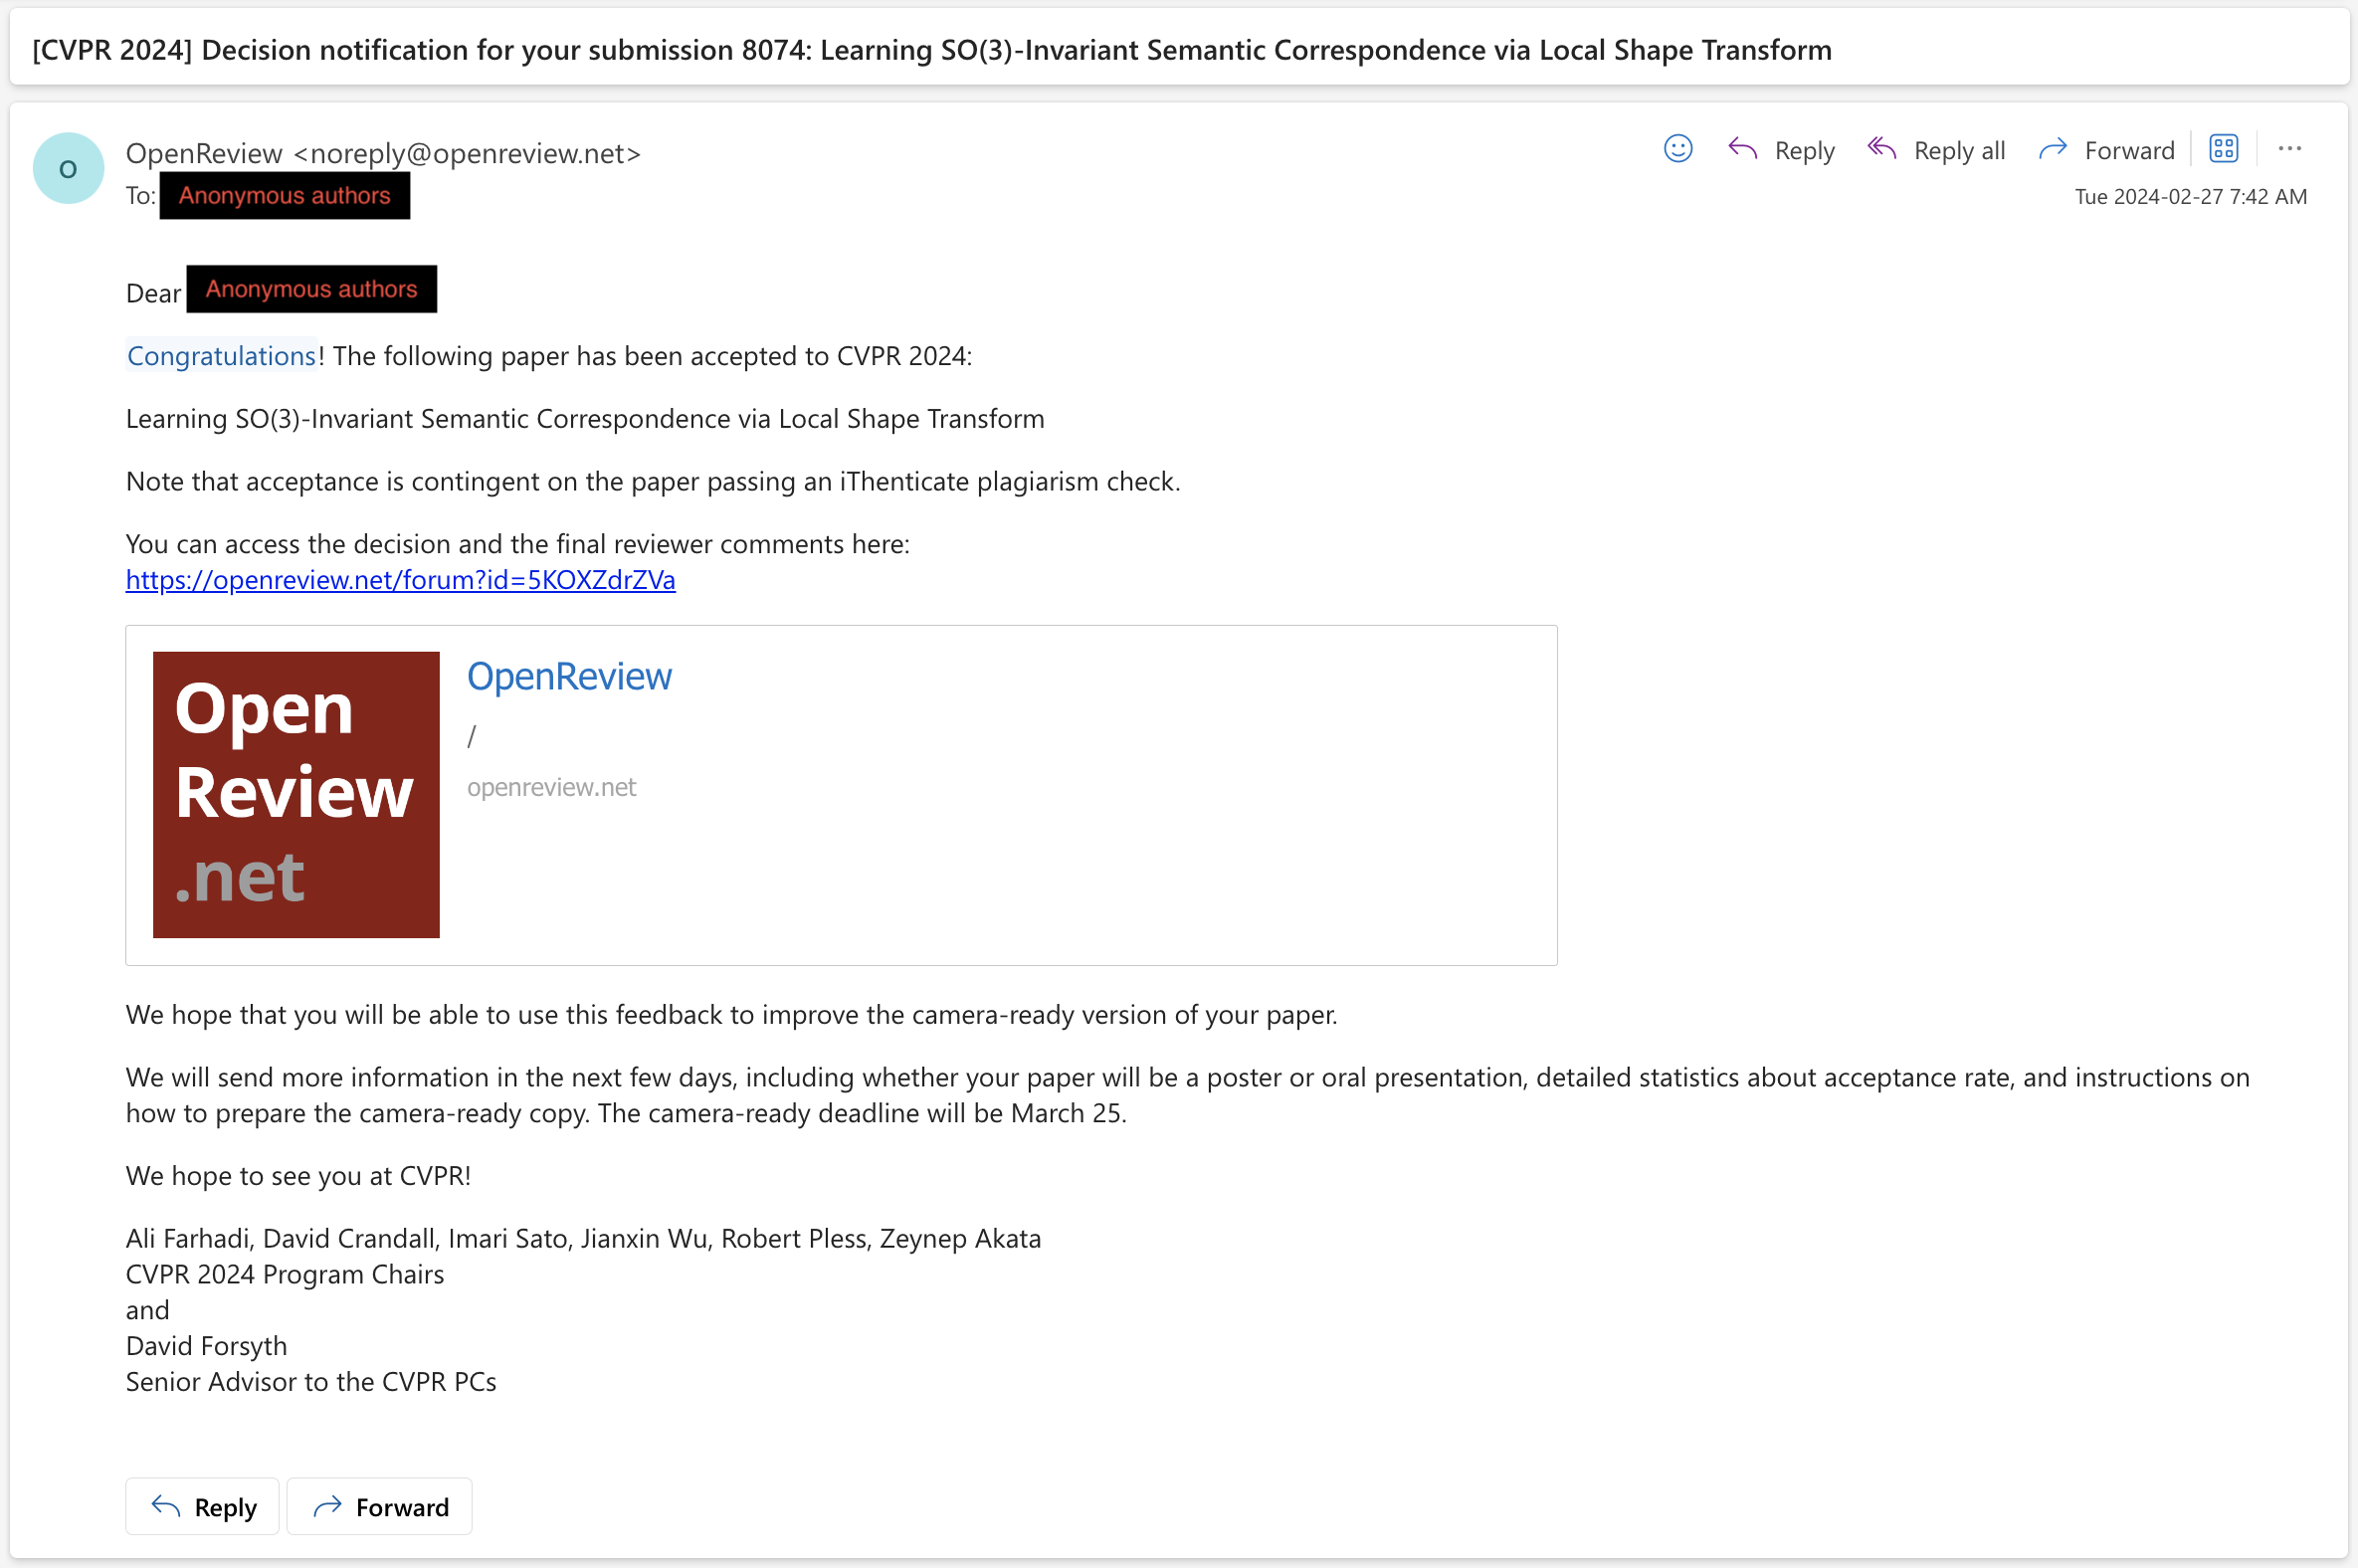}
    \end{center}
\label{fig:supp_acceptance}
\end{figure}
