# Supplementary material for: Learning SO(3)-Invariant Semantic Correspondence via Local Shape Transform
Source: arXiv:2404.11156 source file (2024-04-20)
Supplement: Supplementary file 2 [file supp_pck_keypointnet_i.tex]

\begin{figure}[h]
    \begin{center}
        \includegraphics[width=1.0\linewidth]{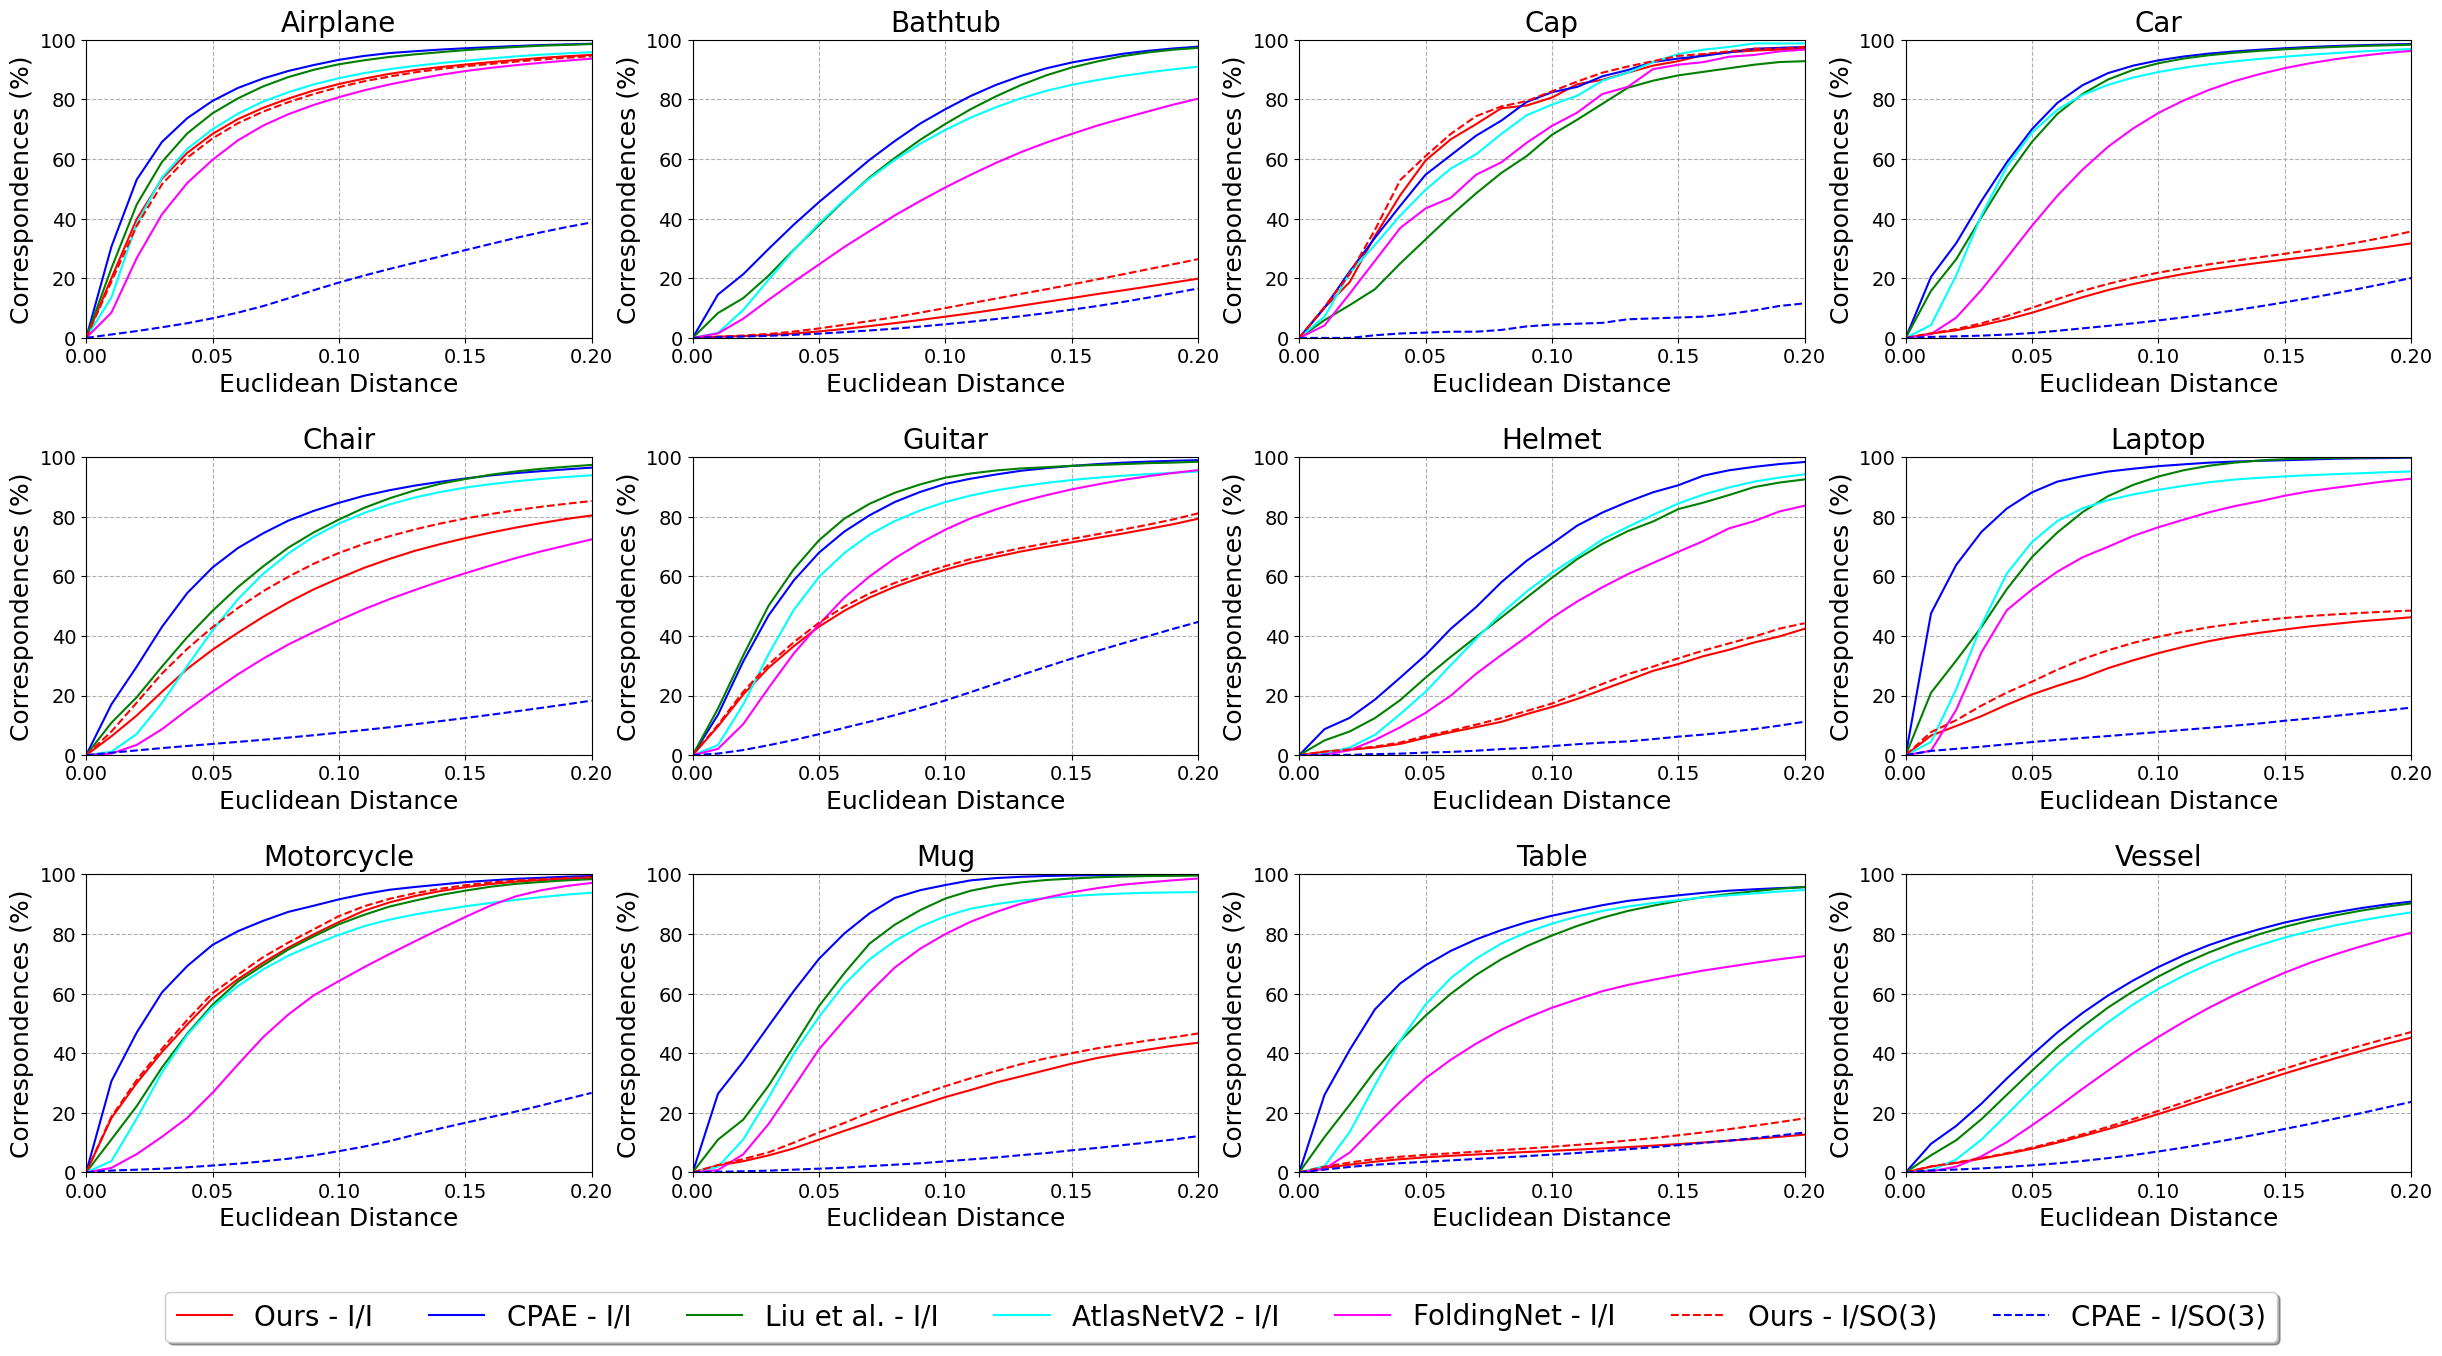}
    \end{center}
      \caption{\textbf{Correspondence accuracy for 12 categories in the KeypointNet dataset.}
}
\label{fig:supp_pck}
\end{figure}
