# Supplementary material for: Learning SO(3)-Invariant Semantic Correspondence via Local Shape Transform
Source: arXiv:2404.11156 source file (2024-04-20)
Supplement: Supplementary file 4 [file a_pck.tex]

\section{Additional results on KeypointNet with I/I and I/SO(3)}
\begin{figure}[h]
    \begin{center}
        \includegraphics[width=1.0\linewidth]{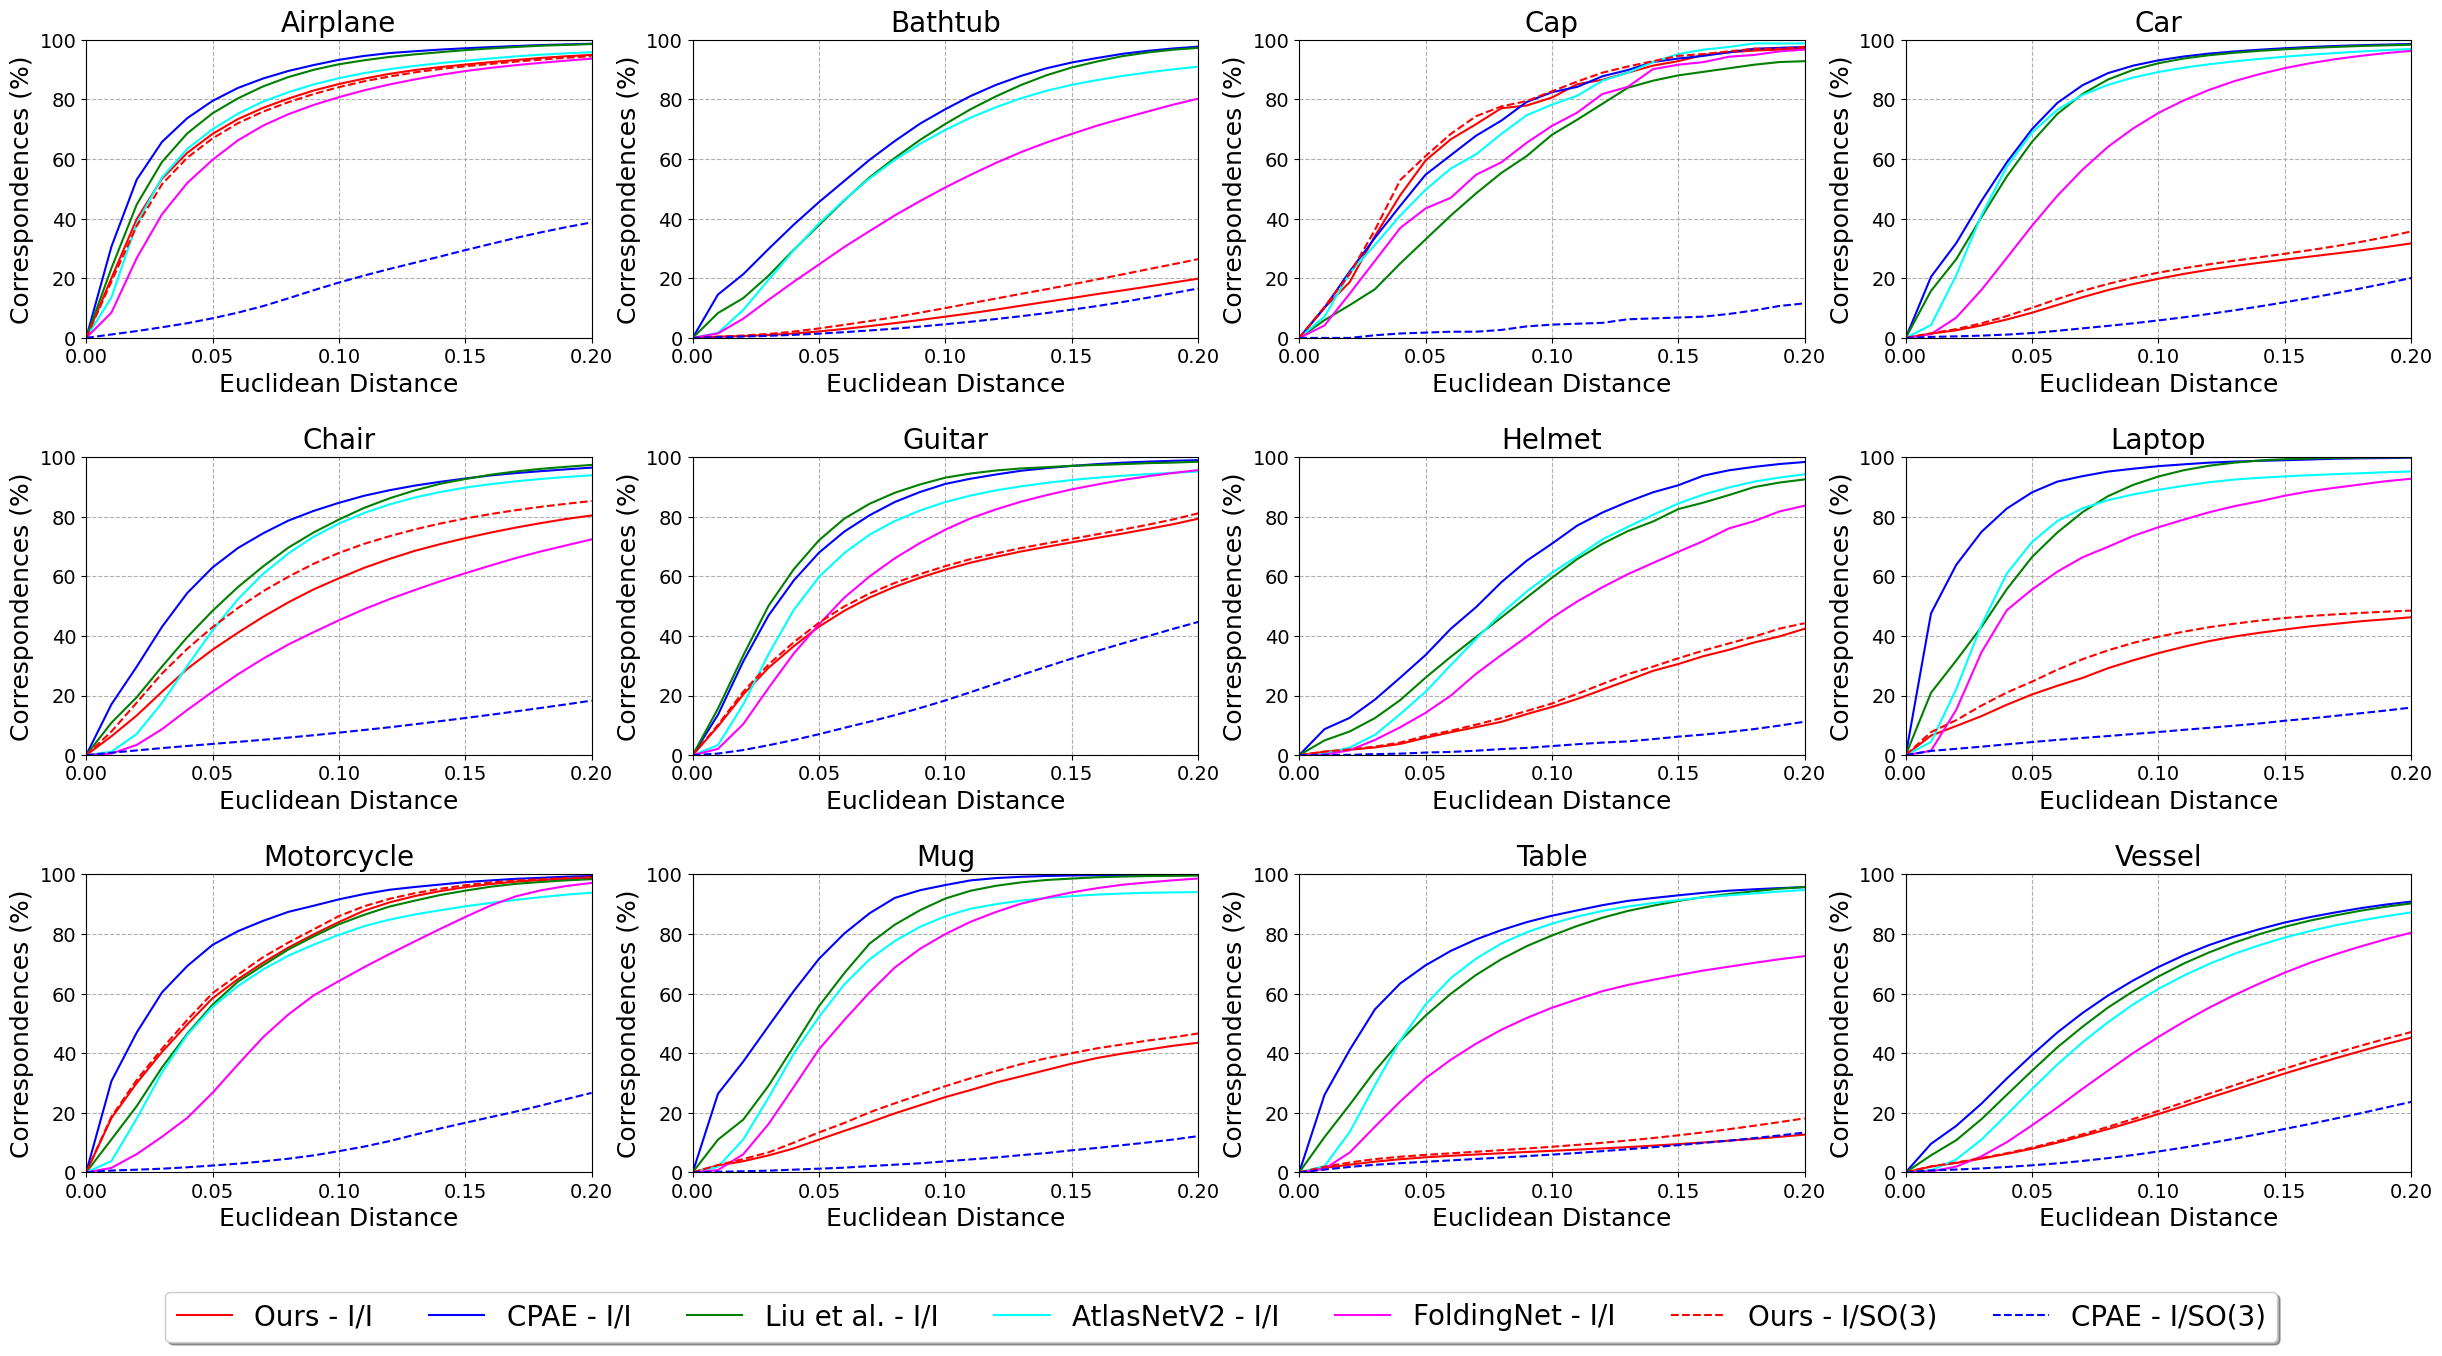}
    \end{center}
      \caption{\textbf{Correspondence accuracy for 12 categories in the KeypointNet dataset.}
}
\label{fig:supp_pck}
\end{figure}

In this section, we provide the results of baseline methods~\citep{deprelle2019learning, yang2018foldingnet, liu2020learning, cheng2021learning} and ours evaluated on the KeypointNet dataset, but under the I/I setting used by previous methods, as shown in Figure~\ref{fig:supp_pck}.
Note that under the I/I setting, the input shape pairs are perfectly aligned both at train and test time - which is an unrealistic setting in practice.
For CPAE~\cite{cheng2021learning} and ours, we also include the results under the I/SO(3) setting to visualize the performance difference between the two evaluation settings.
It can be seen that while the drop in performance for CPAE from I/I to I/SO(3) setting is drastic, the difference is negligible in \methodName, demonstrating the robustness of our SO(3) correspondence establishment scheme against arbitrary rotations.
While \methodName is not always competitive on all datasets, it is impractical to expect perfectly aligned shapes in real-world situations; on the realistic setting of SO(3) evaluation, \methodName consistently shows the best results.
