# Supplementary material for: Learning SO(3)-Invariant Semantic Correspondence via Local Shape Transform
Source: arXiv:2404.11156 source file (2024-04-20)
Supplement: Supplementary file 5 [file d_additional_qual.tex]

\section{Additional qualitative results.}
We provide additional qualitative results which were not included in our manuscript due to space constraints, as shown in Figures~\ref{fig:supp_part_motor},~\ref{fig:supp_part_guitar}, and~\ref{fig:supp_part_airplane}.
It can be seen that under especially large intra-class variation, part segmentation label transfer using \methodName often yields unsatisfactory results.
\input{assets/figures/tex/supp_qual_part_label_transfer_motorcycle}
\begin{figure*}[h]
    \begin{center}
        \includegraphics[width=\linewidth]{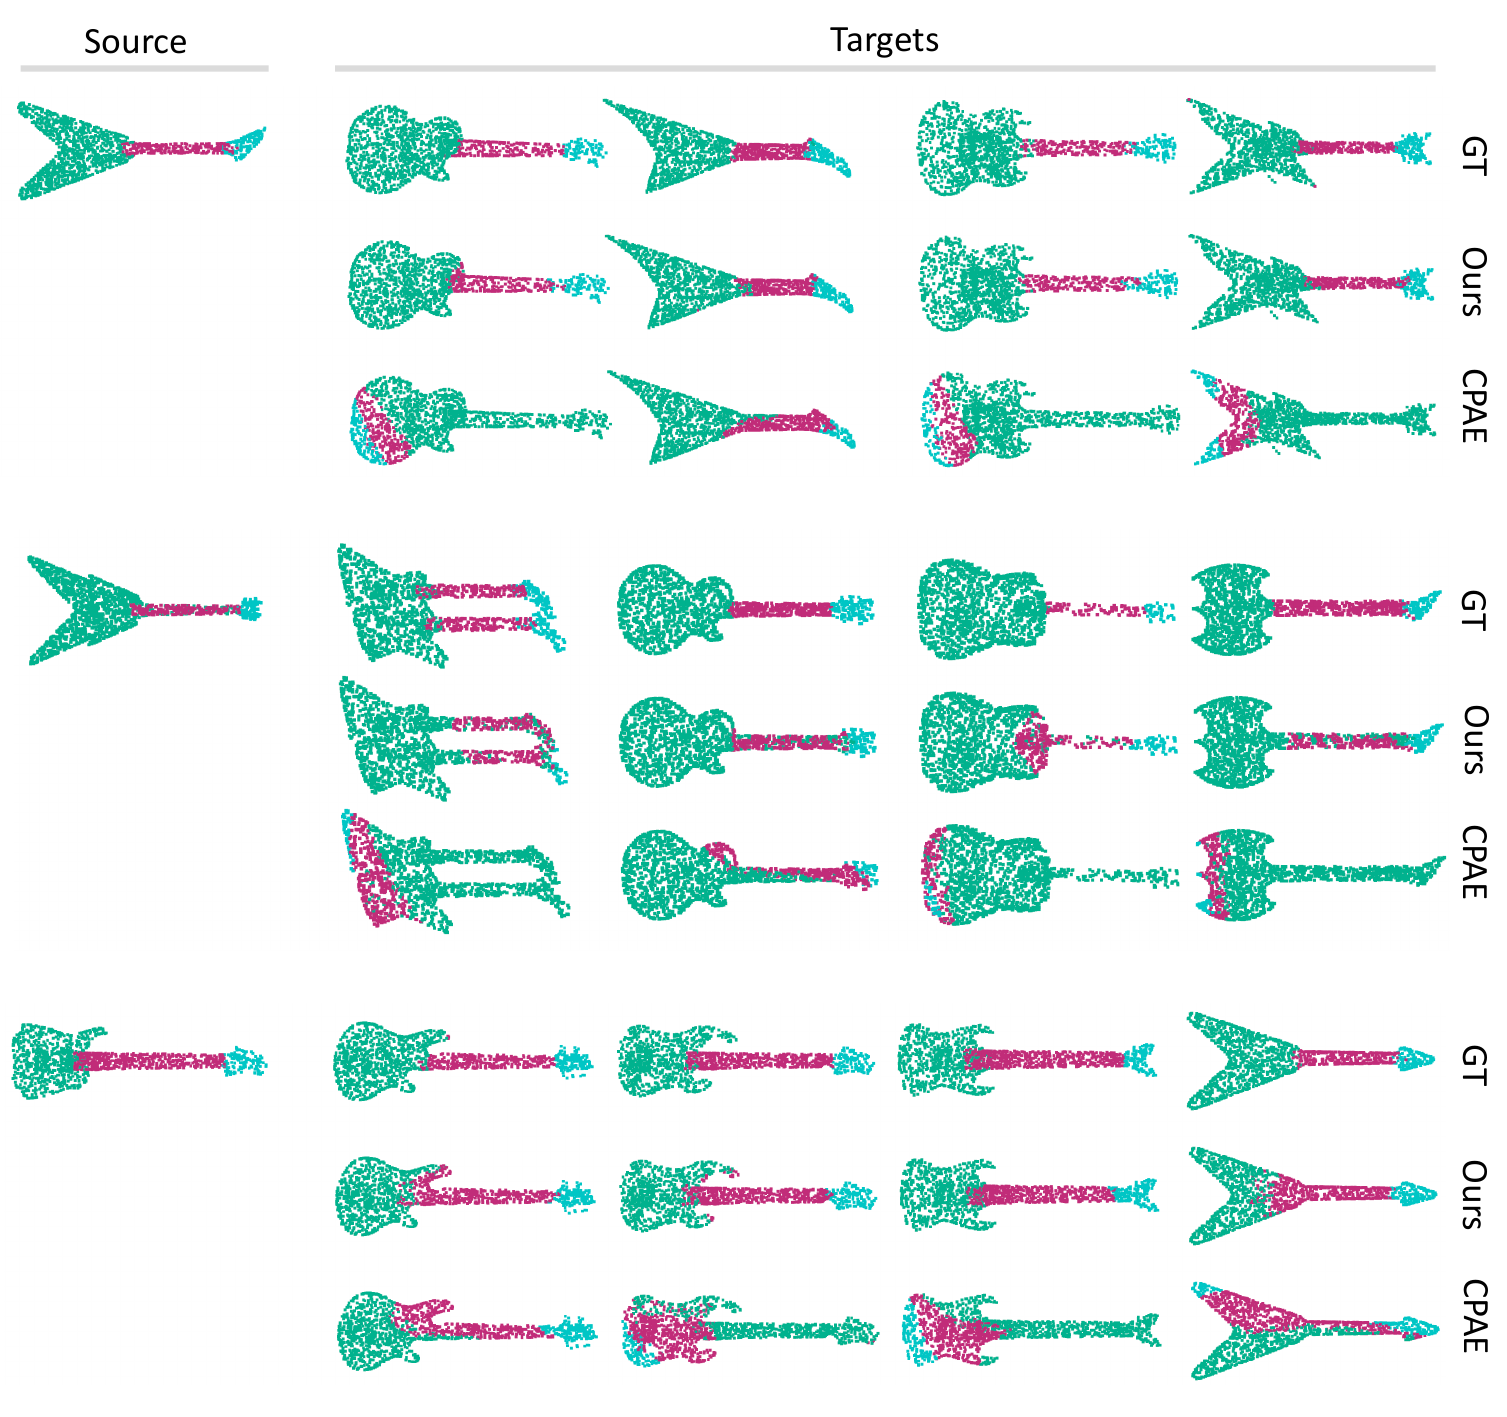}
    \end{center}
      \caption{\textbf{Qualitative results of part label transfer on the guitar class in the ShapeNet part dataset~\cite{shapenetpart}.} Note that the input shapes were arbitrarily rotated, differently for each target column, but have been aligned for better visibility of part label transfer results.
      \methodName shows to outperform CPAE~\cite{cheng2021learning} consistently, showing a high resemblance to ground truth results.
}
\label{fig:supp_part_guitar}
\end{figure*}
\input{assets/figures/tex/supp_qual_part_label_transfer_airplane}
